# Supplementary material for: Auxilio and Beyond: Comparative Evaluation, Usability, and Design Guidelines for Head Movement-based Assistive Mouse Controllers
Source: arXiv:2210.04483 source file (2026-01-11)
Supplement: Supplementary file 1 [file Usability_analysis_of_Auxilio_using_System_Usability_Scale_SUS.pdf]

\* Required

- Mark only one oval.

Mark only one oval.

Mark only one oval.

|                   |                       |                       |                       |                       |                       |                |
|-------------------|-----------------------|-----------------------|-----------------------|-----------------------|-----------------------|----------------|
|                   | 1                     | 2                     | 3                     | 4                     | 5                     |                |
| Strongly Disagree | <input type="radio"/> | <input type="radio"/> | <input type="radio"/> | <input type="radio"/> | <input type="radio"/> | Strongly Agree |



8. I found the system very cumbersome to use. \*

*Mark only one oval.*

|                   | 1                     | 2                     | 3                     | 4                     | 5                     |                |
|-------------------|-----------------------|-----------------------|-----------------------|-----------------------|-----------------------|----------------|
| Strongly Disagree | <input type="radio"/> | <input type="radio"/> | <input type="radio"/> | <input type="radio"/> | <input type="radio"/> | Strongly Agree |

9. I felt very confident using the system. \*

*Mark only one oval.*

|                   | 1                     | 2                     | 3                     | 4                     | 5                     |                |
|-------------------|-----------------------|-----------------------|-----------------------|-----------------------|-----------------------|----------------|
| Strongly Disagree | <input type="radio"/> | <input type="radio"/> | <input type="radio"/> | <input type="radio"/> | <input type="radio"/> | Strongly Agree |

10. I needed to learn a lot of things before I could get going with this system. \*

*Mark only one oval.*

|                   | 1                     | 2                     | 3                     | 4                     | 5                     |                |
|-------------------|-----------------------|-----------------------|-----------------------|-----------------------|-----------------------|----------------|
| Strongly Disagree | <input type="radio"/> | <input type="radio"/> | <input type="radio"/> | <input type="radio"/> | <input type="radio"/> | Strongly Agree |

---

This content is neither created nor endorsed by Google.

Google Forms
